# Supplementary material for: High-efficiency energy harvesting based on nonlinear Hall rectifier
Source: arXiv:2211.17219 source file (2023-07-31)
Supplement: Supplementary file 1 [file Supplemental_Materials.pdf]

# Supplemental material for "High-efficiency energy harvesting based on nonlinear Hall rectifier"

Yugo Onishi[1] and Liang Fu[1]

[1] *Department of Physics, Massachusetts Institute of Technology, Cambridge, MA 02139, USA*

(Dated: July 31, 2023)

## I. GENERAL EXPRESSION FOR POWER TRANSFER/RECTIFICATION EFFICIENCY

In this section, we provide the general expressions for the power transfer/rectification efficiency, $\vartheta_t, \vartheta_c$.

For general systems where $\sigma_{yxx} = -\sigma_{xyx}$ does not necessarily hold and $\sigma_{xxxx}$ is not negligible, the input power $P_{\text{in}}$ and the work done at the load resistance $W_L^{\text{dc}}, W_L^{\text{ac}}$ are given by

$$W_L^{\text{dc}} = \Omega \frac{\sigma_L \sigma_{yxx}^2}{4(\sigma_{yy}+\sigma_L)^2} E_x^4, \tag{1}$$

$$W_L^{\text{ac}} = \frac{1}{2} W_L^{\text{dc}}, \tag{2}$$

$$P_{\text{in}} = \Omega \left[ \frac{1}{2}\sigma_{xx}E_x^2 + \frac{3}{8}\left(\sigma_{xxxx} + \frac{-\sigma_{xyx}\sigma_{yxx}}{\sigma_{yy}+\sigma_L}\right) E_x^4 \right]. \tag{3}$$

Therefore, we obtain the efficiency $\vartheta_t, \vartheta_c$ as

$$\vartheta_t = \left(-\frac{\sigma_{yxx}}{\sigma_{xyx}}\right) \frac{r_L}{(1+r_L)^2} \frac{1}{\alpha + r_L/(1+r_L)} \frac{E_x^2}{E_1^2 + E_x^2}, \tag{4}$$

$$\vartheta_c = \frac{2}{3}\vartheta_t, \tag{5}$$

where $\alpha, E_1, r_L$ are defined as following:

$$\alpha = -\frac{\sigma_{xxxx}\sigma_{yy}}{\sigma_{xyx}\sigma_{yxx}}, \tag{6}$$

$$E_1 = \frac{2}{\sqrt{3}} E_0 \sqrt{\frac{1+\alpha}{\alpha + r_L/(1+r_L)}}, \tag{7}$$

$$E_0 = \left(\frac{\sigma_{xxxx}}{\sigma_{xx}} - \frac{\sigma_{xyx}\sigma_{yxx}}{\sigma_{yy}\sigma_{xx}}\right)^{-1/2}, \tag{8}$$

$$r_L = \frac{R_L}{R_{yy}}. \tag{9}$$

Note that $\vartheta_t, \alpha$ are reduced to the ones in the main text when $\sigma_{yxx} = -\sigma_{xyx}$. It should be also noted that, when $\sigma_{yxx} \neq -\sigma_{xyx}$, higher order terms are necessary to ensure $\vartheta_t \leq 1$. This is because $\sigma_{yxx}, \sigma_{xyx}$ contribute to the Joule heating $Q/\Omega = \boldsymbol{j}\cdot\boldsymbol{E}$ as $(\sigma_{yxx}+\sigma_{xyx})E_x^2 E_y$, and they are negative when $E_y$ is applied in a certain direction. To ensure $Q \geq 0$ (and hence $\vartheta_t \leq 1$), one needs higher order contributions to $Q$ such as $\sigma_{yyxx}E_y^2 E_x^2$.

## II. ESTIMATED EFFICIENCY FOR NONLINEAR HALL MATERIALS

Based on available parameters in the literature, we can roughly estimate the efficiency for known nonlinear Hall materials. For most materials, we assume here that $\sigma_{yxx} = -\sigma_{xyx}$ and $\sigma_{xxxx}$ and higher order conductivity are negligible. In this case, the power transfer efficiency $\vartheta_t$ can be rewritten in a more useful form. Given the Hall voltage $V_y$ observed when the current $I_x$ is applied in $x$-direction, $\vartheta_t(I_x, r_L)$ at the current $I_x$ and the external load $R_L = r_L R_{yy}$ can be calculated as

$$\vartheta_t(I_x, r_L) = \frac{1}{1+r_L}\left(\frac{1+r_L}{r_L}\frac{4R_{xx}R_{yy}I_x^2}{3V_y(I_x)^2} + 1\right)^{-1}, \tag{10}$$

where $R_{xx}, R_{yy}$ are the resistance in $x$ and $y$ direction, and $R_L$ is the load resistance. In deriving Eq. (10), we assumed that the applied $I_x$ and $E_x$ are small enough so that the linear relation between the voltage and the current in $x$-direction $V_x, I_x$ holds, $V_x = R_{xx} I_x$. In particular, the maximum efficiency with respect to $r_L$ for a fixed $I_x$ is given at $r_L = r_L^*$:

$$\max_{r_L} \vartheta_t(I_x, r_L) = \vartheta_t(I_x, r_L^*) = \left(\frac{r_L^*}{1+r_L^*}\right)^2 \frac{3V_y(I_x)^2}{4R_{xx}R_{yy}I_x^2}, \tag{11}$$

$$r_L^* = \sqrt{\frac{4R_{xx}R_{yy}I_x^2}{4R_{xx}R_{yy}I_x^2 + 3V_y(I_x)^2}}. \tag{12}$$

With these formulas, one can calculate the maximum efficiency for a given $I_x$ with $R_{xx}, R_{yy}$ and the corresponding Hall voltage $V_y(I_x)$.

Another useful expression is the following:

$$\vartheta_t(I_x, r_L) = \frac{1}{1+r_L}\left(\frac{1+r_L}{r_L}\frac{4\sigma_{xx}E_x^2}{3\sigma_{yy}E_y^2} + 1\right)^{-1}. \tag{13}$$

$$\max_{r_L} \vartheta_t(I_x, r_L) = \vartheta_t(I_x, r_L^*) = \left(\frac{r_L^*}{1+r_L^*}\right)^2 \frac{3\sigma_{yy}E_y^2}{4\sigma_{xx}E_x^2}, \tag{14}$$

$$r_L^* = \sqrt{\frac{4\sigma_{xx}E_x^2}{3\sigma_{yy}E_y^2 + 4\sigma_{xx}E_x^2}}. \tag{15}$$

This expression allows us to estimate $\vartheta_t$ with two ratios $\sigma_{xx}/\sigma_{yy}$ and $E_x/E_y$. Defining the Hall angle $\Theta_H$ as $\tan\Theta_H = E_y/E_x$, we obtain the expression Eq. (23) in the main text.

Assuming $\sigma_{yxx} = -\sigma_{xyx}$ and $V_x \propto I_x$, we can useEq. (11) or (14) to estimate $\max_{r_L} \vartheta_t$ for several nonlinear Hall materials in literature. The results are summarized in Table I. Among them, $WTe_2$ is estimated to have the highest efficiency as high as $\max_{r_L} \vartheta_t = 4.3\,\%$.

TABLE I. Estimated efficiency for nonlinear Hall materials. Except for $T_d$-$MoTe_2$, the efficiency $\max_{r_L} \vartheta_t(I_x, r_L)$, is estimated with Eq. (11) and the parameters $I_x, V_y$ and $R_{xx}$ listed in the table, assuming $R_{xx} = R_{yy}$ and $\sigma_{yxx} = -\sigma_{xyx}$. $T_d$-$MoTe_2$ is estimated with Eq. (14) assuming $E_y/E_x = 2.4$ and $\sigma_{xx}/\sigma_{yy} = 4$.

| Material | Temperature(K) | Frequency(Hz) | $I_x(\mu A)$ | $V_y(\mu V)$ | Assumed $R_{xx}(\Omega)$ | $\max_{r_L} \vartheta_t(I_x, r_L)$ |
|---|---|---|---|---|---|---|
| Bulk $WTe_2$ [1] | 1.4-4.2 | 110 | 4000 | 2.0 | 0.0010 | 0.043 |
| $T_d$-$MoTe_2$ [2] | 2-40 | 17-277 | 5000 | 40 | - | 0.030 [a] |
| $Cd_3As_2$ [1] | 1.4-4.2 | 110 | 4000 | 1.0 | 0.0050 | 0.00047 |
| Bilayer $WTe_2$ [3] | 10-100 | 10-1000 | 1.0 | 200 | 5000 | 0.00030 |
| $MnBi_2Te_4$(+BP) (unpublished) | 0-20 | 6GHz | 10 | 300 | 10000 | 0.0000017 |
| $Ce_3Bi_4Pd_3$ [4] | 1.4-4.2 | 110 | 10000 | 0.80 | 0.030 | 0.0000013 |
| Corrugated bilayer graphene [5] | 1.5-15 | 77 | 0.10 | 1.0 | 4000 | 0.0000012 |

[a] Eq. (14) is used for the estimation. The used Hall ratio is $E_y/E_x = 2.4$.


[1] O. O. Shvetsov, V. D. Esin, A. V. Timonina, N. N. Kolesnikov, and E. V. Deviatov, Nonlinear Hall Effect in Three-Dimensional Weyl and Dirac Semimetals, JETP Letters **109**, 715 (2019).

[2] A. Tiwari, F. Chen, S. Zhong, E. Drueke, J. Koo, A. Kaczmarek, C. Xiao, J. Gao, X. Luo, Q. Niu, Y. Sun, B. Yan, L. Zhao, and A. W. Tsen, Giant c-axis nonlinear anomalous Hall effect in Td-MoTe2 and WTe2, Nature Communications **12**, 2049 (2021).

[3] Q. Ma, S.-Y. Xu, H. Shen, D. MacNeill, V. Fatemi, T.-R. Chang, A. M. Mier Valdivia, S. Wu, Z. Du, C.-H. Hsu, S. Fang, Q. D. Gibson, K. Watanabe, T. Taniguchi, R. J. Cava, E. Kaxiras, H.-Z. Lu, H. Lin, L. Fu, N. Gedik, and P. Jarillo-Herrero, Observation of the nonlinear Hall effect under time-reversal-symmetric conditions, Nature **565**, 337 (2019).

[4] S. Dzsaber, X. Yan, M. Taupin, G. Eguchi, A. Prokofiev, T. Shiroka, P. Blaha, O. Rubel, S. E. Grefe, H.-H. Lai, Q. Si, and S. Paschen, Giant spontaneous hall effect in a nonmagnetic weyl–kondo semimetal, Proceedings of the National Academy of Sciences **118**, e2013386118 (2021).

[5] S.-C. Ho, C.-H. Chang, Y.-C. Hsieh, S.-T. Lo, B. Huang, T.-H.-Y. Vu, C. Ortix, and T.-M. Chen, Hall effects in artificially corrugated bilayer graphene without breaking time-reversal symmetry, Nature Electronics **4**, 116 (2021).
